# Supplementary material for: XekRung Technical Report
Source: arXiv:2605.00072 source file (2026-11-06)
Supplement: Supplementary file 1 [file appendix.tex]

\section{Appendix}

\subsection{Extended Evaluation Results}\label{app:extended_eval}
